# Supplementary material for: Modeling nonlocal behavior in epidemics via a reaction-diffusion system incorporating population movement along a network
Source: arXiv:2205.04868 source file (2022-05-09)
Supplement: Supplementary file 1 [file 5_Appendix.tex]

\section*{Appendix}
\label{sec:appendix}

\setcounter{equation}{0}
\setcounter{figure}{0}
\setcounter{table}{0}
\makeatletter
